# Supplementary material for: Decentralized Implicit Differentiation
Source: arXiv:2403.01260 source file (2024-03-02)
Supplement: Supplementary file 1 [file QP.tex]

\section{Derivation for QPs}\label{appendix:QP}

In this section, as an exercise, we derive all relevant relationships in the general case of subproblems defined by QPs with linear constraints, and linear coupling constraints. That is, the general problem writes
\begin{align*}
    \min_{x_i} & \sum_i^N x_i^TP_ix_i + c_i^Tx_i\\
    \text{s.t. }& A_ix_i-b_i \preccurlyeq 0, \ i = 1, ...,\ N \\ 
   &  M\mathbf{x}-d = 0
\end{align*}
where the matrices $P_i$ are PSD, and the global coupling matrix $M = [m_1, m_2, ..., m_N]$. 

\paragraph{Local Jacobians} Let us take $\theta_i = (c_i, b_i)$ as the parameters we are interested in evaluating the sensitivity towards.
The local problems after writing the partial Lagrangian are $(i=1...N):$
\begin{align*}
    \min_{x_i} &\ x_i^TP_ix_i + c_i^Tx_i + \nu^Tm_ix_i\\
    \text{s.t. }& A_ix_i-b_i \preccurlyeq 0
\end{align*}
Writing $z_i = (x_i, \lambda_i)$ where $\lambda_i$ is the \textit{local} dual variable, and $\bar{\theta}_i = [\theta_i, \nu]$, the KKT matrix $g_i$ writes
$$
g_i = 
\begin{bmatrix}
c_i + m_i^T\nu + A_i^T\lambda_i + P_ix_i\\
diag(\lambda_i)(A_ix_i-b_i)
\end{bmatrix}, 
$$
and we have
$$
\partial_{z_i}g_i(z_i, \bar{\theta}_i) =
\begin{bmatrix}
    P_i & A_i^T\\
    diag(\lambda_i)A_i & diag(A_ix_i-b_i)
\end{bmatrix} \in \mathbbm{R}^{(n+l) \times (n+l)}.
$$
Given the chosen parameters, we have
$$
\partial_{\bar{\theta}_i}g_i = 
\begin{bmatrix}
    I & 0 & m_i^T \\
    0 & -diag(\lambda_i) & 0
\end{bmatrix} \in \mathbbm{R}^{(n+l) \times (n+l+\Lambda)}.
$$
Once we have computed these quantities, we  can solve
\begin{align}
    \partial_{\bar{\theta}_i}x_i &= - (\partial_{z_i}g_i(z_i, \bar{\theta}_i))^{-1}\partial_{\bar{\theta}_i}g_i \\
    & = [\partial_{\theta_i}x_i, \partial_{\nu}x_i]
\end{align}

\paragraph{Consensus} We are now in position to compute $\partial_{\pmb{\theta}}\nu$ given Eq.~\eqref{eq:consensus}. We can gather all local jacobians computed above and,
rewriting this equation with the appropriate variables, 
\begin{equation}
    \partial_{\pmb{\theta}}\nu = -(M\partial_\nu \mathbf{x})^{-1}M\partial_{\pmb{\theta}}\mathbf{x}
\end{equation}
Under the current assumptions of independence of parameters and local primal variables, we note that $\partial_{\theta_j}x_i = 0$ for $ i \neq j$. Note that the matrix $M\partial_\nu \mathbf{x} \in \mathbbm{R}^{\Lambda \times \Lambda}$.

\paragraph{Updating local Jacobians}
The final step is to compute the total derivative of the local variables wrt local parameters according to Eq.~\eqref{eq:update_local}:

\begin{align}
   D_{\theta_i}x_i^\star(\theta_i, \nu) = \partial_{\theta_i} x_i^\star + \partial_{\nu}x_i^\star \partial_{\theta_i}\nu 
\end{align}
