# Supplementary material for: Decentralized Implicit Differentiation
Source: arXiv:2403.01260 source file (2024-03-02)
Supplement: Supplementary file 2 [file Self-dual.tex]

\section{Derivation via self-dual embeddings}\label{appendix:self-dual}

\subsection{Cone constraints}
General cone constraints present a different challenge. Indeed, according to Amos, we cannot easily differentiate through the KKT because of the cone constraints. \textbf{I DON'T UNDERSTAND WHY THAT IS THE CASE YET, BUT LET'S WALK WITH THIS ASSUMPTION FOR NOW}

If this is true, we need a generalization of the KKT condition to differentiate through so that the framework is applicable to also SOCP, SDP, etc. To enable this, we borrow from Ye, Besutti, O'Donohue, Agrawal and Amos (5 different papers). These papers rely on an embedding proposed by Ye to implicitly define the solution. Basically, it is another set of conditions that the solution needs to satisfy, and relies on a few properties.

I will illustrate my thinking roughly here, and polish the text later.

First of all, the above logic still applies. Namely, we can write the Lagrangian containing the objective function and the coupling constraint. At optimality, every local problem solves the local objective + part of the term that involves the coupling constraint, s.t. local constraints. So, basically, the proposed logic still applies. 

Second, we differentiate locally, also as exposed. \textbf{Note: If the local problem is a cone program, we can differentiate through it given methods exposed in mentioned papers (Amos, Agrawal). It is important to state that the only thing we do, locally, is differentiate as is already known in the literature - but we differentiate with the objective being the augmented Lagrangian, and wrt extended parameters}. 

We have so far expressed how to compute the coupling jacobian in the case of equality or inequality constraints. This logic simply relied on differentiating through the KKT conditions. However, it is not as easy to do if the coupling constraint is of the form
\begin{align*}
h_i(x) \preccurlyeq_{\mathcal{K_i}} 0, \ i =1, ... \Lambda
\end{align*}
with $\mathcal{K}$ being a second-order cone, a semi definite cone, exponential cone, etc. This said, we should intuitively still be able to perform a similar operation, that is, express the gradient of the dual coupling variable as a function of individual gradients, and correct the local gradients on this basis.

\subsubsection{Homogeneous self-dual embedding}

Similarly to the above mentioned papers, we propose to build an embedding of the coupling constraint and coupling dual variable: 
\begin{align*}
Q = \begin{bmatrix} 
0 & H(x) \\
- H(x)^T & 0
\end{bmatrix}
\end{align*},
where $H(x)^T = [h_1(x), ... h_\Lambda(x)]$. \textbf{If we have a solution} (here the goal is not to find a solution, we assume we have an appropriate solution to the problem), then we construct two vector $u, v$ such that $u = (\lambda, 1), v = (s, 0)$, where $\lambda = [\lambda_1, ... \lambda_\Lambda]$ is the vector of dual variables associated with the coupling constraints and $s = [s_1, ... s_\Lambda]$ is the primmal slack variable associated to those cone constraints. This implies
\begin{itemize}
    \item $Qu = v$ (i.e. the coupling constraint is satisfied as well as the associated complementary slackness condition)
    \item $ u \in \bar{\mathcal{K}}, \bar{\mathcal{K}} = \mathcal{K}^\star \times \mathbb{R}_+$; $v \in \bar{\mathcal{K}}^\star, \in \bar{\mathcal{K}}^\star = \mathcal{K} \times \mathbb{R}_+$. Therefore, both $u, v$ belong to cones that are mutually dual! Indeed, the nonnegative orthant is self dual \textbf{I think?}. 
    \item $u^Tv = 0$, i.e. $u, v$ belong to complementary vector spaces in $\mathbb{R}^\Lambda$
\end{itemize}

Given those properties, we can use the theorem of Moreau that enables decomposition of an element of a hilbert space over the conic complementary set. Namely, we have that
\begin{align*}
    z = u - v\\
    u = \Pi_{\bar{\mathcal{K}}} z, v = - \Pi_{\bar{\mathcal{K}}^\star} z\\ 
    \Rightarrow \Pi_{\bar{\mathcal{K}}} = I - \Pi_{\bar{\mathcal{K}}^\star}
\end{align*}

For simplicity, we will denote $\Pi_{\bar{\mathcal{K}}}$ simply by $\Pi$ in the remainder of the document. 

Therefore, we can rewrite the condition that $u, v$ satisfy as
\begin{align*}
    Q\Pi z + (I - \Pi)z = 0 \\ 
    ((Q - I)\Pi + I) z = 0 = \mathcal{R}(z)
\end{align*}
$\mathcal{R}(z)$ denotes the residual map. It is supposed to be $0$ for any solution embedded in the above way.

\subsubsection{Derivation through the embedding}
The above embedding provides a map $\mathcal{R}(z)$ that is different from the KKT conditions but is differentiable. Once it is constructed, the only thing we need is to do is apply the same mechnanics as before. 

The only thing we want to recover is the Jacobian $D_\theta \lambda =[I, 0] D\Pi (z) D_\theta z = [\Pi_{\mathcal{K}^\star},\ 0]D_\theta z$ (\textbf{note} that we are projecting on the dual cone, because we want to recover the dual variables).  Therefore, we can recover the gradient of the dual variable by projecting the gradient of $z$. 

We apply the implicit differentiation theorem, again. 

\begin{align*}
    \partial_\theta z = - (\partial_z \mathcal{R}(z))^{-1} \partial_\theta \mathcal{R}(z)
\end{align*}

We can analyze both terms in this equation:
\begin{itemize}
    \item $\partial_z \mathcal{R}(z) = \partial_z Q \Pi z + (Q- I) \partial_z (\Pi z) + I$\\
    \item $\partial_\theta \mathcal{R}(z) = \partial_\theta Q \Pi z$
\end{itemize}

Computing $\partial_z Q$ is the new part here. Let's note that $\partial_z x_i(\theta, \lambda(\theta)) = \partial_\lambda x_i \partial_z \lambda = \partial_\lambda x_i [I, 0] D\Pi$, as $\lambda = [I, 0] \Pi z$. This allows the derivation of the matrix $Q$ wrt $z$. The rest should not be an issue. Similarly, we can compute $\partial_\theta Q$ by taking the derivatives directly for each component of the matrix.

\subsubsection{Ensuring invertibility}

As we have seen, we need the last component of $z$ to ensure complementary slackness but we never recover the information at that level. Indeed, $\lambda = [I, 0] \Pi z$. Therefore, we only need ``all the rows but the last one'' of the inverse of the residual map. I have some hints indeed that it might now always be differentiable \textbf{why?}. Therefore, we can construct only the first row of the inverse of the matrix (by block decomposition), multiply it by the RHS, and then project on the dual cone without ever thinking about the last component of $z$.
