# Supplementary material for: Decentralized Implicit Differentiation
Source: arXiv:2403.01260 source file (2024-03-02)
Supplement: Supplementary file 3 [file NonSeparableConstraints.tex]

\section{Non Separable Constraints}\label{appendix:non-separable}
