# Supplementary material for: Decentralized Implicit Differentiation
Source: arXiv:2403.01260 source file (2024-03-02)
Supplement: Supplementary file 4 [file SuppFigs.tex]

\section{Supplementary Figures}\label{appendix:supp_figs}

\begin{figure}[ht]
    \centering
    \includegraphics[width=.5\textwidth]{Figures/Scaling/ρ_fixed_th0.8_speedup.pdf}
    \caption{Scaling of the computational gain for a fixed number of coupling constraints $\Lambda=2$, and for different sizes of subproblems, with the central problem represented as a sparse matrix.}
    \label{supp_fig:scaling_sparse}
\end{figure}

\begin{figure}[ht]
    \centering
    \includegraphics[width=.4\textwidth]{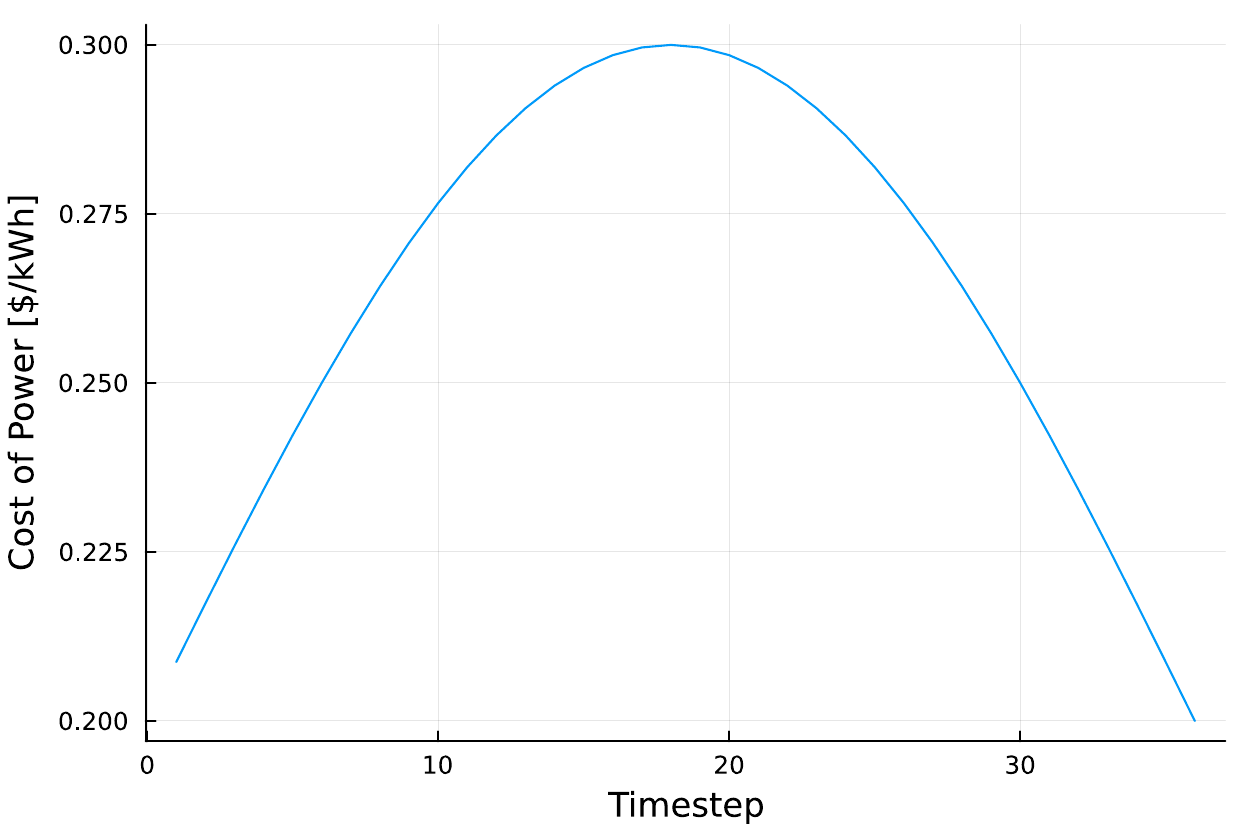}
    \caption{Caption}
    \label{supp_fig:cost}
\end{figure}
